# Supplementary material for: Instability-driven Oscillations of Elastic Microfilaments
Source: arXiv:1808.01583 ancillary file (2018-11-24)
Supplement: Supplementary file 1 [file Ling2018_supp.pdf]

# Instability-driven Oscillations of Active Microfilament

## Supplemental Material

Feng Ling, Hanliang Guo, and Eva Kanso\*  
 Department of Aerospace and Mechanical Engineering,  
 University of Southern California, Los Angeles, California 90089, USA  
 (Dated: August 5, 2018)

### I. LIST OF SUPPLEMENTAL MOVIES

- S1 Motion of filament under tip follower force of  $F_a = 75$  subject to *non-planar* perturbation starting from the straight equilibrium. The resulting spinning motion has a locked curvature at steady state.
- S2 Motion of filament under tip follower force of  $F_a = 75$  subject to *planar* perturbation starting from the straight equilibrium. The resulting flapping motion is confined to a plane.
- S3 Robustness of transition from straight to 3D spinning. At  $F_a = 180$ , spinning is stable. Initial configuration is set by adding a small out-of-plane perturbation to the planar solution. The basin of attraction of these spinning solutions seems to consist of all non-planar perturbations.
- S4 Robustness of transition from 3D spinning to 2D flapping. At  $F_a = 200$ , flapping is stable. Initial configuration is set to the spinning solution obtained at  $F_a = 185$ . At  $F_a = 200$ , the filament trajectory converges to in-plane motion. The basin of attraction of these planar flapping solutions seems to consist of all initial perturbations.
- S5 Bead-spring models under *non-planar* perturbations at  $F_a = 5$ . As we increase the number of links from 2 to 6, stable 2D flapping motions emerge from 3D spinning motions.

### II. NUMERICAL METHODS AND VALIDATIONS

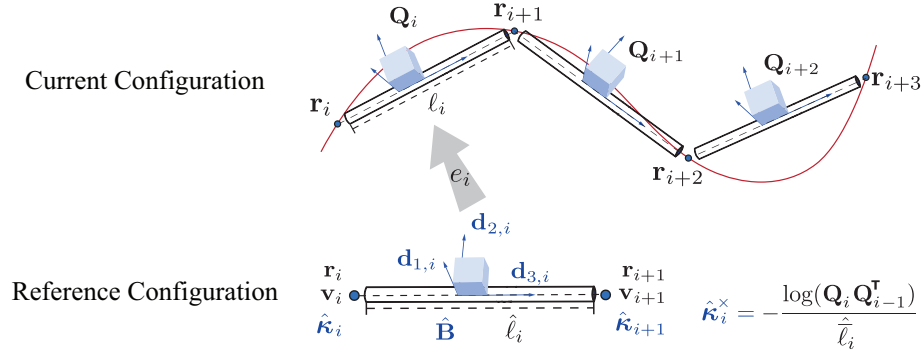

FIG. 1: Discretization of elastic filament

We discretize the filament's centerline into  $n + 1$  vertices  $\mathbf{r}_1, \dots, \mathbf{r}_{n+1}$  and  $n$  straight edges  $\ell_i = \mathbf{r}_{i+1} - \mathbf{r}_i$ , where  $i = 1, \dots, n$ , in the spirit of [1] and [2]; see Fig. 1. The unit tangent to edge  $i$  is defined as  $\mathbf{t}_i = \ell_i / \ell_i$  where  $\ell_i = \|\ell_i\|$ . Inextensibility is enforced weakly by considering large tensile stiffness  $S = EA$  along the filament's centerline. That is to say,  $\mathbf{t}$  is allowed to experience slight extension or compression, inducing a local axial strain  $\mathbf{s}_i = (\ell_i / \hat{\ell}_i) \mathbf{t}_i - \mathbf{d}_3^i$ , where  $\hat{\ell}_i$  is a strain-free reference configuration length. The linear velocities  $\mathbf{v}_1, \dots, \mathbf{v}_{n+1}$  are assigned to vertices. The body frames are naturally assigned to edges, so is the rotation matrix  $\mathbf{Q}$ ; we let  $\{\mathbf{d}_{1,i}, \mathbf{d}_{2,i}, \mathbf{d}_{3,i} = \mathbf{t}_i\}$  and  $\mathbf{Q}_i$  denote

\* kanso@usc.edu

the discrete representation of these quantities. Here, we defined the rotation matrix  $\mathbf{Q}$  using the convention  $\mathbf{x}_b = \mathbf{Q}\mathbf{x}$ , where  $\mathbf{x}_b$  is the position vector expressed in body-frame coordinates (see appendix A). Throughout this work, the subscript  $b$  will be used to emphasize when vectors are represented in the body frame.

The skew-symmetric matrix  $\boldsymbol{\kappa}^\times = (\partial\mathbf{Q}/\partial s)^\top \mathbf{Q}$  can be expressed in the body frame by a change of basis as  $\boldsymbol{\kappa}_b^\times = \mathbf{Q}\boldsymbol{\kappa}^\times \mathbf{Q}^\top = \mathbf{Q}(\partial\mathbf{Q}/\partial s)^\top$ . The solution to the differential equation  $\boldsymbol{\kappa}_b^\times = \mathbf{Q}(\partial\mathbf{Q}/\partial s)^\top$  is of the form  $\mathbf{Q}(s + \Delta s) = \exp(-\boldsymbol{\kappa}_b^\times \Delta s)\mathbf{Q}(s)$ , given that the curvature stays constant in the region  $\Delta s$ . We can thus define the discrete curvature  $\boldsymbol{\kappa}_{b,i}^\times$  such that  $\mathbf{Q}_i = \exp(-\boldsymbol{\kappa}_{b,i}^\times \bar{\ell}_i)\mathbf{Q}_{i-1}$ , leading to

$$\boldsymbol{\kappa}_{b,i}^\times = -\frac{\log(\mathbf{Q}_i \mathbf{Q}_{i-1}^\top)}{\bar{\ell}_i}. \quad (1)$$

Here,  $\bar{\ell}_i = \frac{1}{2}(\ell_{i-1} + \ell_i)$  is a ‘Voronoi’ integration domain spanning from the midpoint of the previous edge to that of the next edge. Remember that this definition of discrete curvature is only defined at an *interior* vertex  $i = 2, \dots, n$ .

To obtain the bending dynamics of the filament, we first use equation (3) of the main text to solve for the internal elastic force  $\mathbf{N}_i$  in the body frame of the current geometric configuration of the filament,

$$\mathbf{N}_{b,i} = \mathbf{t}_{b,i} \times \left\{ \mathcal{D}[\mathbf{B}_{b,i} \boldsymbol{\kappa}_{b,i}] + \mathcal{A}[\underbrace{(\boldsymbol{\kappa}_{b,i} \bar{\ell}_i) \times (\mathbf{B}_{b,i} \boldsymbol{\kappa}_{b,i})}_{\text{frame transport}}] \right\} + (EA)\mathbf{s}_{b,i}. \quad (2)$$

Here, the finite difference operator  $\mathcal{D}$  and discrete average operator  $\mathcal{A}$  take quantities on  $i$ -th and  $(i+1)$ -th vertices as inputs and output quantities on the  $i$ -th edge ( $i = 1, \dots, n$ ). Since  $\bar{\ell}_i$  and  $\boldsymbol{\kappa}_{b,i}$  are only defined at interior vertices, we need to pad trivial (zero) quantities for boundary vertices ( $i = 1$  and  $n+1$ ). In other words, the  $j$ -th output of  $\mathcal{D}[(\cdot)_i]$  is  $(\cdot)_i \delta_{i,j+1} - (\cdot)_i \delta_{ij}$ . Similarly, the  $j$ -th output of  $\mathcal{A}[(\cdot)_i]$  is  $[(\cdot)_i \delta_{i,j+1} + (\cdot)_i \delta_{ij}]/2$ . Note that inextensibility is enforced weakly by setting the axial component of  $\mathbf{N}_{b,i}$  to be  $(EA)\mathbf{s}_{b,i}$  with a large stiffness  $EA$ .

Next, we invert the force balance in equation (1) using the expression for the fluid force from equation (2) of the main text to get the inertial frame velocity  $\mathbf{v}_i$  of each vertex

$$\mathbf{v}_i = \frac{1}{\gamma\zeta} \left( \mathbf{I} + (\gamma - 1)\mathcal{A}[\mathbf{t}_i] \otimes \mathcal{A}[\mathbf{t}_i] \right) \left( \mathcal{D}[\mathbf{N}_i] - \mathbf{f}_{a,i} \ell_i \right). \quad (3)$$

Here the operators  $\mathcal{D}$  and  $\mathcal{A}$  actually convert  $n$  edge quantities to  $n+1$  vertex quantities unlike in (2).

In the numerical implementation, we solve (2) and (3) in the strain-free reference configuration. Therefore we need to adjust all quantities expressed in the current geometric configuration to the strain-free reference state (we use the hat notation  $\hat{(\cdot)}$  to denote the latter). Provided that cross-sections retain their circular shapes at all times, we only need to insert a local dilation scalar  $e_i = \ell_i/\hat{\ell}_i$  at appropriate places in the discretized equations to ensure consistency. Specifically, due to the conservation of volume of an infinitesimal volume element, a dilation in edge length translates to a shrinkage of cross sectional area; namely, we have  $\ell_i A_i = \hat{\ell}_i \hat{A}_i$  which implies that  $A_i = \hat{A}_i/e_i$ . Consequently, the discrete bending/twisting rigidity tensor  $\hat{\mathbf{B}}_i$  and tensile stiffness  $\hat{S}_i$  in the strain-free reference configuration are related to  $\mathbf{B}_i$  and  $S_i$  in the current configuration via  $\mathbf{B}_i = \hat{\mathbf{B}}_i/e_i^2$  and  $S_i = \hat{S}_i/e_i$ . All length quantities need to include a factor of  $e_i$  when converted to the strain-free reference configuration. In addition, because we used the integration domain  $\bar{\ell}_i$  in the momentum equation (2), we need to average all quantities that vary with arc-length over the voronoi region  $\bar{\ell}_i$ . For example, the bending rigidity  $\mathbf{B}$  and dilation factor  $e$  are averaged over  $\bar{\ell}_i$  using

$$\hat{\mathcal{B}}_i = \frac{\hat{\mathbf{B}}_i \hat{\ell}_i + \hat{\mathbf{B}}_{i-1} \hat{\ell}_{i-1}}{2\hat{\ell}_i}, \quad \hat{\mathcal{E}}_i = \frac{e_i \hat{\ell}_i + e_{i-1} \hat{\ell}_{i-1}}{2\hat{\ell}_i}.$$

When adjusting the generalized curvature with respect to the dilation factor, we write  $\boldsymbol{\kappa}_i = \hat{\boldsymbol{\kappa}}_i/\mathcal{E}_i$ .

We use standard time integrators for stiff equations (MATLAB’s `ode15s`) to solve (3) and propagate the filament position  $\mathbf{r}_i$  forward in time. To closed the system, we enforce the clamped boundary condition by fixing  $\mathbf{r}_1 = \mathbf{0}$  and  $\mathbf{t}_1 = \mathbf{e}_3$ , while leaving the free end unconstrained.

We test our numerical method on the deflection and buckling behavior of a cantilever beam submerged in viscous fluid. Since the steady state shape of a cantilever beam under transverse tip load would remain the same in the presence of fluid drag, it is sound to compared our simulation results with the linear Euler-Bernoulli theory at a large  $t$  (in the absence of local filament shear). Indeed we observe first order convergence of our deflected filament at  $t = 20L^4\mu/B$  as we increase spatial resolution; See Fig. 2. Similarly, since the onset of Euler buckling of a cantilever beam under axial compression at one end should also remain equal regardless of the surrounding medium,

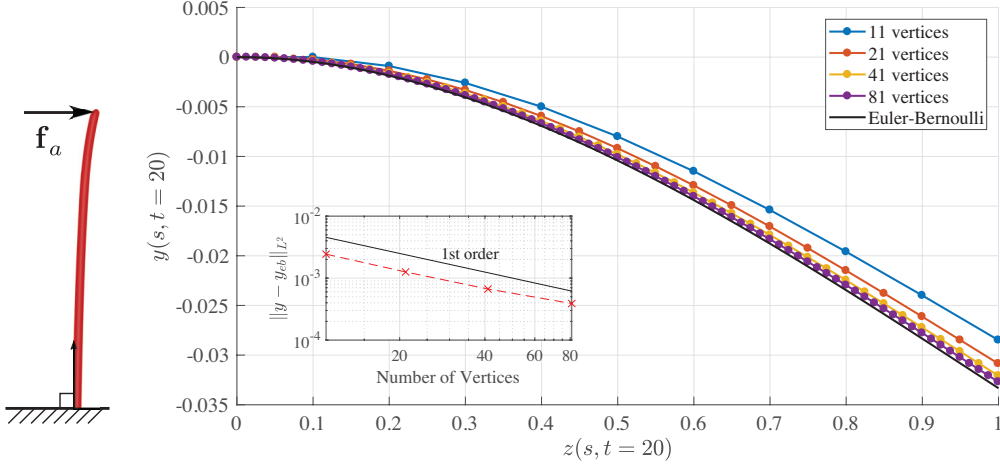

**FIG. 2: Cantilever Deflection in Stokes' Regime.** A cantilever beam subjected to a tip load of  $0.1B/L^3$  submerged in viscous fluids is simulated and its state at  $t = 20L^4\mu/B$  is shown to converge to Euler-Bernoulli theory.

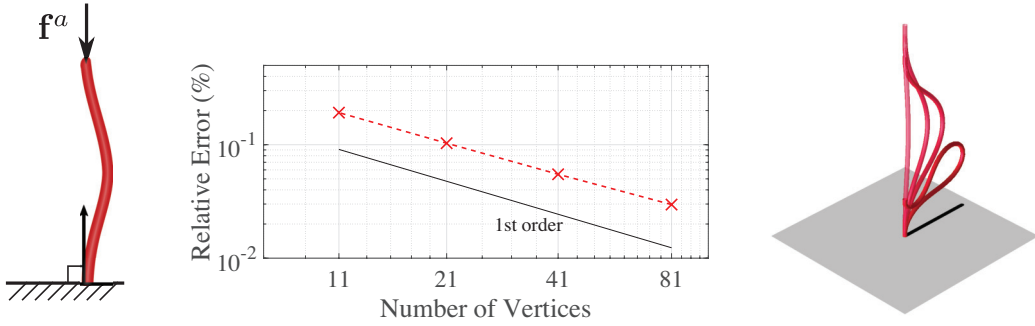

**FIG. 3: Euler Buckling in Stokes' Regime.** Euler buckling of a clamped-clamped beam is simulated in viscous fluids under vertical compressive tip loads. The critical force thresholds converge to the theoretical value in the limit of spatial refinement. Snapshots of the actual buckled shapes are shown for a tip load of  $80B/L^2$ .

we compare the threshold of buckling event with the linear theory result of  $F_{crit} = 4\pi^2(B/L^2)$ . Again we observe first order convergence in the relative error in the limit of spatial refinement. Moreover, our numerical simulation also give the *nonlinear* buckled shape of the filament.

To conclude, we note that the actual algorithm developed is slightly more general in that we can allow twist in the filament following the methods in [1]. In the presence of properly-chosen applied twists, the algorithm correctly exhibit the localized helical buckling instability as well as the Mitchell instability [3–7]; See Fig. 4.

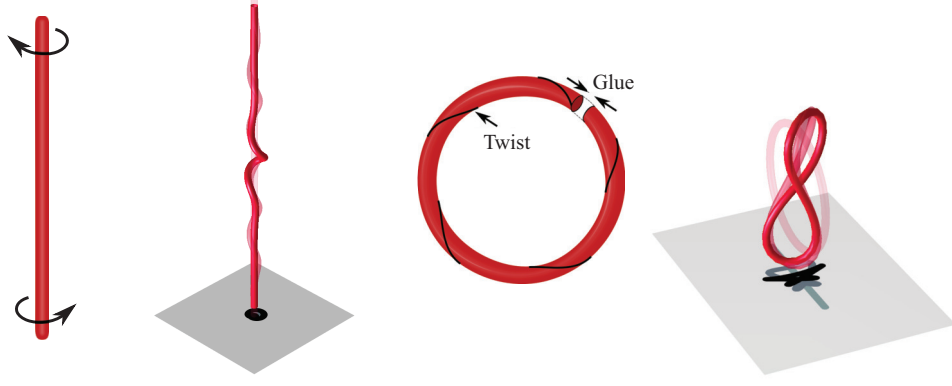

**FIG. 4: Helical Buckling and Mitchell Instability in Stokes' Regime.** Helical buckling occurs when an elastic rod is twisted at its ends to a sufficient degree. Mitchell instability describes the buckling behavior when a sufficiently twisted rod is glued at its two ends. In both case, the time snapshots from our simulation prove that we recover the desired behavior. Quantitative verifications are omitted for brevity.

### III. DERIVATION OF LINEARIZED EQUATIONS

Starting from the force and moment balance and constitutive relations

$$0 = \frac{\partial \mathbf{N}}{\partial s} + \mathbf{f}_a + \mathbf{f}_h$$

$$0 = \frac{\partial \mathbf{M}}{\partial s} + \mathbf{t} \times \mathbf{N}$$

$$\mathbf{M} = \mathbf{B}\boldsymbol{\kappa}$$

Here  $\mathbf{B} = B \cdot \text{diag}(1, 1, 2)$  is the constant bending rigidity, and  $\boldsymbol{\kappa} = k_1 \mathbf{d}_1 + k_2 \mathbf{d}_2$  is the generalized curvature vector. Here we assume there are no twist moments. The usual curvature  $\kappa$  and torsion  $\tau$  of the filament as a space curve in  $\mathbb{R}^3$  can be computed as

$$\kappa(s) = \|\boldsymbol{\kappa}(s)\| = \sqrt{k_1^2 + k_2^2}, \quad (4)$$

$$\tau(s) = \frac{\partial}{\partial s} \left[ \cos^{-1} \left\langle \frac{\boldsymbol{\kappa}(s)}{\kappa(s)}, \frac{\boldsymbol{\kappa}(0)}{\kappa(0)} \right\rangle \right] = \frac{\partial}{\partial s} \left[ \tan^{-1} \frac{k_2}{k_1} \right] = -\frac{\partial}{\partial s} \left[ \tan^{-1} \frac{k_1}{k_2} \right] := \frac{\partial \theta}{\partial s}. \quad (5)$$

Without loss of generality, we assume that at time  $t = 0$ , the curvature vector  $\boldsymbol{\kappa}(0) = \kappa(0)\mathbf{b}$  is aligned with the binormal vector  $\mathbf{b}$  in Frenet-Serret frame. This also means that for a planar (*torsion-free*) filament, the generalized curvature is the *torsion-free* Darboux vector  $\mathbf{D} = \kappa\mathbf{b} \equiv k_2\mathbf{d}_2$ . In general, the Darboux vector is given by  $\mathbf{D} = \kappa\mathbf{b} - \tau\mathbf{t}$ .

In this parallel transport (Bishop) frame ( $\mathbf{d}_1, \mathbf{d}_2, \mathbf{d}_3 \equiv \mathbf{t}$ ), which is equivalent to the material frame without twist, we have

$$\frac{\partial}{\partial s} \begin{bmatrix} \mathbf{d}_1 \\ \mathbf{d}_2 \\ \mathbf{d}_3 \equiv \mathbf{t} \end{bmatrix} = \boldsymbol{\kappa} \times \begin{bmatrix} \mathbf{d}_1 \\ \mathbf{d}_2 \\ \mathbf{d}_3 \equiv \mathbf{t} \end{bmatrix} = \begin{bmatrix} 0 & 0 & -k_2 \\ 0 & 0 & k_1 \\ k_2 & -k_1 & 0 \end{bmatrix} \begin{bmatrix} \mathbf{d}_1 \\ \mathbf{d}_2 \\ \mathbf{d}_3 \equiv \mathbf{t} \end{bmatrix}.$$

Consider the moment balance in (4) and substitute the constitutive relation for the moment to get

$$\mathbf{0} = (\mathbf{B}\boldsymbol{\kappa})_s + \mathbf{t} \times \mathbf{N}$$

$$\mathbf{0} = B \left[ k_{1,s} \mathbf{d}_1 + k_{2,s} \mathbf{d}_2 + \cancel{k_1(k_2\mathbf{t})} + k_2(-k_1\mathbf{t}) \right] + \mathbf{t} \times \mathbf{N}$$

$$\mathbf{0} = \mathbf{t} \times \mathbf{0} = B (\mathbf{t} \times [k_{1,s} \mathbf{d}_1 + k_{2,s} \mathbf{d}_2]) + \mathbf{t} \times (\mathbf{t} \times \mathbf{N})$$

$$\mathbf{0} = B [k_{1,s} \mathbf{d}_2 - k_{2,s} \mathbf{d}_1] + \underbrace{(\mathbf{t} \cdot \mathbf{N}) \mathbf{t}}_{=: \Lambda} - \underbrace{(\mathbf{t} \cdot \mathbf{t}) \mathbf{N}}_{\text{inextensible}} \overset{1}{\mathbf{N}}$$

where  $\Lambda$  is a lagrange multiplier for the inextensibility constraint. Note that to match the equations derived using Frenet-Serret frame in 2D, we need to set  $\Lambda \mapsto \Lambda - B\kappa^2$ . Take the derivative of the above equation with respect to arclength  $s$ , using the notation  $()_{,s} = \partial()/\partial s$ , we get

$$\begin{aligned} \mathbf{0} &= \mathbf{0}_s = B[k_{1,ss}\mathbf{d}_2 - k_{2,ss}\mathbf{d}_1 + k_{1,s}(k_1\mathbf{t}) - k_{2,s}(-k_2\mathbf{t})] + (\Lambda\mathbf{t})_s - \mathbf{N}_s \\ -\mathbf{f}_h &= B[k_{1,ss}\mathbf{d}_2 - k_{2,ss}\mathbf{d}_1 + (k_1k_{1,s} + k_2k_{2,s})\mathbf{t}] + (\Lambda\mathbf{t})_s + \mathbf{f}_a \\ \zeta[\mathbf{t}\mathbf{t}^\top + \gamma(\mathbf{d}_1\mathbf{d}_1^\top + \mathbf{d}_2\mathbf{d}_2^\top)]\mathbf{v} &= -\mathbf{f}_h = B[k_{1,ss}\mathbf{d}_2 - k_{2,ss}\mathbf{d}_1 + \kappa\kappa_s\mathbf{t}] + \Lambda_s\mathbf{t} + \Lambda(k_2\mathbf{d}_1 - k_1\mathbf{d}_2) + \mathbf{f}_a \end{aligned} \quad (6)$$

and  $\zeta$  the drag coefficient with  $\gamma$  representing its anisotropy. Now if we invert the drag coefficients and make use of only an axial applied force ( $\mathbf{f}_a = -f_a\mathbf{t}$ ), we can rewrite the above as

$$\mathbf{v} = \frac{\mathbf{d}_1}{\zeta\gamma}(-Bk_{2,ss} + k_2\Lambda) + \frac{\mathbf{d}_2}{\zeta\gamma}(Bk_{1,ss} - k_1\Lambda) + \frac{\mathbf{t}}{\zeta}[B\kappa\kappa_s + \Lambda_s - f_a]$$

Now, normalize the equation by filament length  $L$  and bending rigidity  $B$ , we require  $s \mapsto \frac{1}{L}s$ , curvatures  $k_i \mapsto Lk_i$ , tension force  $\Lambda \mapsto \frac{B}{L^2}\Lambda$ , force density  $f_a \mapsto \frac{B}{L^3}f_a$ , and velocity  $\mathbf{v} \mapsto \frac{B}{\zeta L^3}\mathbf{v}$ . In dimensionless form, we have

$$\mathbf{v} = \mathbf{d}_1(-k_{2,ss} + k_2\Lambda) + \mathbf{d}_2(k_{1,ss} - k_1\Lambda) + \gamma\mathbf{t}[\kappa\kappa_s + \Lambda_s - f_a]$$

In order to rewrite the left-hand side in terms of ‘known’ variables ( $k_i, \mathbf{d}_i, \mathbf{t}$ ), we differentiate the above w.r.t.  $s$  again to get, using the notation  $()_t = \partial()/\partial t$ ,

$$\begin{aligned} \mathbf{t}_t = \mathbf{v}_s &= \mathbf{t}[\gamma(\kappa\kappa_{ss} + f_{a,s} + \kappa_s^2 + \Lambda_{ss}) + k_1(-k_1\Lambda + k_{1,ss}) - k_2(k_2\Lambda - k_{2,ss})] + \\ &\quad \mathbf{d}_2[-\Lambda k_{1,s} - k_1\Lambda_s - \gamma k_1(-f_a + \kappa\kappa_s + \Lambda_s) + k_{1,sss}] + \\ &\quad \mathbf{d}_1[\Lambda k_{2,s} + k_2\Lambda_s + \gamma k_2(-f_a + \kappa\kappa_s + \Lambda_s) - k_{2,sss}] \end{aligned}$$

Again from inextensibility constraint  $\mathbf{t} \cdot \mathbf{t}_t = 0$ , so the tangent component of above quantity is 0. Finally, we have the following system of scalar equations

$$0 = \gamma(\kappa\kappa_{ss} + f_{a,s} + \kappa_s^2 + \Lambda_{ss}) - \kappa^2\Lambda + k_1k_{1,ss} + k_2k_{2,ss} \quad (7)$$

$$\mathbf{d}_2 \cdot \mathbf{t}_t = -\Lambda k_{1,s} - k_1\Lambda_s - \gamma k_1(-f_a + \kappa\kappa_s + \Lambda_s) + k_{1,sss} \quad (8)$$

$$\mathbf{d}_1 \cdot \mathbf{t}_t = \Lambda k_{2,s} + k_2\Lambda_s + \gamma k_2(-f_a + \kappa\kappa_s + \Lambda_s) - k_{2,sss}. \quad (9)$$

which we slightly rearrange to get

$$\begin{aligned} 0 &= \gamma(\kappa\kappa_s - f_a + \Lambda_s)_s - \Lambda\kappa^2 + k_1k_{1,ss} + k_2k_{2,ss} \\ -\mathbf{d}_2 \cdot \mathbf{t}_t &= (\Lambda k_1)_s + \gamma k_1(\kappa\kappa_s - f_a + \Lambda_s) - k_{1,sss} \\ \mathbf{d}_1 \cdot \mathbf{t}_t &= (\Lambda k_2)_s + \gamma k_2(\kappa\kappa_s - f_a + \Lambda_s) - k_{2,sss} \end{aligned}$$

The first equation leads to the constraint equation

$$\gamma(\kappa\kappa_s - f_a + \Lambda_s)_s = \Lambda\kappa^2 - k_1k_{1,ss} - k_2k_{2,ss} \quad (10)$$

Take derivative of the last two equations w.r.t.  $s$  to get

$$-(-k_{1,t} + k_2\mathbf{d}_2 \cdot \mathbf{d}_{1,t}) = (\Lambda k_1)_{ss} + \gamma[k_1(\kappa\kappa_s - f_a + \Lambda_s)]_s - k_{1,ssss} \quad (11)$$

$$(k_{2,t} - k_1\mathbf{d}_1 \cdot \mathbf{d}_{2,t}) = (\Lambda k_2)_{ss} + \gamma[k_2(\kappa\kappa_s - f_a + \Lambda_s)]_s - k_{2,ssss} \quad (12)$$

Multiply (11) and (12) by  $k_1$  and  $k_2$ , respectively, to get

$$\begin{aligned} k_1(k_{1,t} - k_2\mathbf{d}_2 \cdot \mathbf{d}_{1,t}) &= k_1(\Lambda k_1)_{ss} + \gamma k_1[k_1(\kappa\kappa_s - f_a + \Lambda_s)]_s - k_1k_{1,ssss} \\ k_2(k_{2,t} - k_1\mathbf{d}_1 \cdot \mathbf{d}_{2,t}) &= k_2(\Lambda k_2)_{ss} + \gamma k_2[k_2(\kappa\kappa_s - f_a + \Lambda_s)]_s - k_2k_{2,ssss} \end{aligned}$$

Take the sum of the above two equations

$$k_1 k_{1,t} + k_2 k_{2,t} = k_1 (\Lambda k_1)_{ss} + \gamma k_1 k_{1,s} (\kappa \kappa_s - f_a + \Lambda_s) + k_1^2 [\Lambda \kappa^2 - k_1 k_{1,ss} - k_2 k_{2,ss}] - k_1 k_{1,ssss} \\ + k_2 (\Lambda k_2)_{ss} + \gamma k_2 k_{2,s} (\kappa \kappa_s - f_a + \Lambda_s) + k_2^2 [\Lambda \kappa^2 - k_1 k_{1,ss} - k_2 k_{2,ss}] - k_2 k_{2,ssss}$$

Upon further simplifications, we arrive at

$$k_1 k_{1,ssss} + k_2 k_{2,ssss} + \kappa \kappa_t = \Lambda_{ss} \kappa^2 + (2 + \gamma) \Lambda_s \kappa \kappa_s + (\Lambda - \kappa^2) (k_1 k_{1,ss} + k_2 k_{2,ss}) \\ + \gamma (\kappa \kappa_s)^2 - \gamma \kappa \kappa_s f_a + \Lambda \kappa^4 \quad (13)$$

Now, multiply (11) and (12) by  $k_2$  and  $k_1$  respectively, to get

$$k_2 (k_{1,t} - k_2 \mathbf{d}_2 \cdot \mathbf{d}_{1,t}) = k_2 (\Lambda k_1)_{ss} + \gamma k_2 [k_1 (\kappa \kappa_s - f_a + \Lambda_s)]_s - k_2 k_{1,ssss} \\ k_1 (k_{2,t} - k_1 \mathbf{d}_1 \cdot \mathbf{d}_{2,t}) = k_1 (\Lambda k_2)_{ss} + \gamma k_1 [k_2 (\kappa \kappa_s - f_a + \Lambda_s)]_s - k_1 k_{2,ssss}$$

The difference of the above two equations yields

$$k_2 k_{1,t} - k_1 k_{2,t} - k_2^2 \mathbf{d}_2 \cdot \mathbf{d}_{1,t} + k_1 \mathbf{d}_1 \cdot \mathbf{d}_{2,t} = k_2 (\Lambda k_1)_{ss} - k_1 (\Lambda k_2)_{ss} - k_2 k_{1,ssss} + k_1 k_{2,ssss} \\ + \gamma k_2 [k_1 (\kappa \kappa_s - f_a + \Lambda_s)]_s - \gamma k_1 [k_2 (\kappa \kappa_s - f_a + \Lambda_s)]_s$$

Upon further simplifications, we get

$$k_2 k_{1,ssss} - k_1 k_{2,ssss} + k_2 k_{1,t} - k_1 k_{2,t} - \kappa^2 (\mathbf{d}_2 \cdot \mathbf{d}_{1,t}) = k_2 (\Lambda_{ss} k_1 + 2 \Lambda_s k_{1,s} + \Lambda k_{1,ss}) \\ - k_1 (\Lambda_{ss} k_2 + 2 \Lambda_s k_{2,s} + \Lambda k_{2,ss}) \\ + \gamma (k_2 k_{1,s} - k_1 k_{2,s}) (\kappa \kappa_s - f_a + \Lambda_s)$$

and

$$k_2 k_{1,ssss} - k_1 k_{2,ssss} + k_2 k_{1,t} - k_1 k_{2,t} - \kappa^2 (\mathbf{d}_2 \cdot \mathbf{d}_{1,t}) = \Lambda (k_2 k_{1,ss} - k_1 k_{2,ss}) \\ + (k_2 k_{1,s} - k_1 k_{2,s}) [\gamma \kappa \kappa_s - \gamma f_a + (2 + \gamma) \Lambda_s] \quad (14)$$

To arrive at the last expression, note that we have

$$k_2 k_{1,t} - k_1 k_{2,t} = -\kappa^2 \theta_t \\ (\mathbf{d}_2 \cdot \mathbf{d}_{1,t}) = \theta_t - \mathbf{n}_t \cdot \mathbf{b}$$

based on  $k_1 = -\kappa \sin \theta$ ,  $k_2 = \kappa \cos \theta$ ,  $\tau = \theta_s$ ,  $\mathbf{d}_1 = \cos \theta \mathbf{b} - \sin \theta \mathbf{n}$ , and  $\mathbf{d}_2 = \sin \theta \mathbf{b} + \cos \theta \mathbf{n}$ . These geometric relations also yield

$$k_1 k_{1,ss} + k_2 k_{2,ss} = \kappa (\kappa_{ss} - \kappa \tau^2) \\ k_1 k_{1,ssss} + k_2 k_{2,ssss} = \kappa (\kappa_{ssss} + \tau (\kappa \tau^3 - 6 \kappa_{ss} \tau - 2 \kappa_s \tau_s - 4 \kappa \tau_{ss}) - 3 \kappa \tau_{ss}^2) \\ k_2 k_{1,s} - k_1 k_{2,s} = -\kappa^2 \tau \\ k_2 k_{1,ss} - k_1 k_{2,ss} = -\kappa (2 \kappa_s \tau + \kappa \tau_s) \\ k_2 k_{1,ssss} - k_1 k_{2,ssss} = \kappa (\tau (4 \kappa_s \tau^2 + 6 \kappa \tau \tau_s - 4 \kappa_{ss}) - 6 \kappa_{ss} \tau_s - 4 \kappa_s \tau_{ss} - \kappa \tau_{ssss})$$

Substituting these relations into (10), (13) and (14), we get

$$\gamma \kappa \kappa_{ss} + \gamma \kappa_s^2 + \gamma (-f_a + \Lambda_s)_s = \Lambda \kappa^2 - \kappa \kappa_{ss} + \kappa^2 \tau^2 \\ \kappa_{ssss} + \tau (\kappa \tau^3 - 6 \kappa_{ss} \tau - 2 \kappa_s \tau_s - 4 \kappa \tau_{ss}) - 3 \kappa \tau_{ss}^2 + \kappa_t = \\ \Lambda_{ss} \kappa + (2 + \gamma) \Lambda_s \kappa_s + (\Lambda - \kappa^2) (\kappa_{ss} - \kappa \tau^2) + \gamma \kappa \kappa_s^2 - \gamma \kappa_s f_a + \Lambda \kappa^3 \\ \tau (4 \kappa_s \tau^2 + 6 \kappa \tau \tau_s - 4 \kappa_{ss}) - 6 \kappa_{ss} \tau_s - 4 \kappa_s \tau_{ss} - \kappa \tau_{ssss} + \kappa \mathbf{n}_t \cdot \mathbf{b} = \\ -\Lambda (2 \kappa_s \tau + \kappa \tau_s) - \kappa^2 \tau [\gamma \kappa \kappa_s - \gamma f_a + (2 + \gamma) \Lambda_s]$$

Expand about straight configuration  $\kappa = \tau = 0$  and linearize in terms of  $\Lambda, \kappa$ , and  $\tau$  to get

$$\begin{aligned} (-f_a + \Lambda_s)_s &= 0 \\ \kappa_{ssss} + \kappa_t - \Lambda \kappa_{ss} &= 0 \\ 0 &= 0 \end{aligned}$$

That is to say, the last equation is trivially satisfied and the torsion is not featured in the linear equations. The linear equations only capture 2D deformations.

- 
- [1] Bergou M, Wardetzky M, Robinson S, Audoly B, Grinspun E. Discrete elastic rods. In: ACM transactions on graphics (TOG). vol. 27. ACM; 2008. p. 63.
  - [2] Gazzola M, Dudte LH, McCormick AG, Mahadevan L. Dynamics of soft filaments that can stretch, shear, bend and twist. arXiv preprint. 2016;.
  - [3] Coyne J. Analysis of the formation and elimination of loops in twisted cable. IEEE Journal of Oceanic Engineering. 1990;15(2):72–83.
  - [4] Van der Heijden G, Thompson J. Helical and localised buckling in twisted rods: a unified analysis of the symmetric case. Nonlinear dynamics. 2000;21(1):71–99.
  - [5] Neukirch S, Van Der Heijden G, Thompson J. Writhing instabilities of twisted rods: from infinite to finite length. Journal of the Mechanics and Physics of Solids. 2002;50(6):1175–1191.
  - [6] Van der Heijden G, Neukirch S, Goss V, Thompson J. Instability and self-contact phenomena in the writhing of clamped rods. International Journal of Mechanical Sciences. 2003;45(1):161–196.
  - [7] Goriely A. Twisted elastic rings and the rediscoveries of Michell’s instability. Journal of Elasticity. 2006;84(3):281–299.

### Appendix A: Rotation Group Conventions

Consider an inertial frame ( $\mathbf{e}_i$ ) and a body frame ( $\mathbf{d}_i$ ),  $i = 1, 2, 3$ . Define the rotation matrix  $\mathbf{Q}$  as the operator that transforms vectors from inertial frame to body frame. We have

$$\mathbf{e}_i = \mathbf{Q} \mathbf{d}_i, \quad (\text{A1})$$

where

$$\mathbf{Q} = \begin{bmatrix} -\mathbf{d}_1^\top & - \\ -\mathbf{d}_2^\top & - \\ -\mathbf{d}_3^\top & - \end{bmatrix}. \quad (\text{A2})$$

A vector  $\mathbf{x}$  can be represented in the inertial frame or the director body frame:  $\mathbf{x} = x_i \mathbf{e}_i = x_{b,i} \mathbf{d}_i$ . To find the relationship between coordinates  $X_i$  and  $x_i$ , rewrite

$$\begin{aligned} x_i \mathbf{e}_i &\equiv \begin{bmatrix} | & | & | \\ \mathbf{e}_1 & \mathbf{e}_2 & \mathbf{e}_3 \\ | & | & | \end{bmatrix} \begin{pmatrix} x_1 \\ x_2 \\ x_3 \end{pmatrix} = \mathbb{I} \begin{pmatrix} x_1 \\ x_2 \\ x_3 \end{pmatrix} = \mathbf{Q}^\top \mathbf{Q} \begin{pmatrix} x_1 \\ x_2 \\ x_3 \end{pmatrix} \\ &= \begin{bmatrix} | & | & | \\ \mathbf{d}_1 & \mathbf{d}_2 & \mathbf{d}_3 \\ | & | & | \end{bmatrix} \mathbf{Q} \begin{pmatrix} x_1 \\ x_2 \\ x_3 \end{pmatrix} =: \begin{bmatrix} | & | & | \\ \mathbf{d}_1 & \mathbf{d}_2 & \mathbf{d}_3 \\ | & | & | \end{bmatrix} \begin{pmatrix} x_{b,1} \\ x_{b,2} \\ x_{b,3} \end{pmatrix} \equiv x_{b,i} \mathbf{d}_i \end{aligned} \quad (\text{A3})$$

Thus, we get  $\mathbf{x}_b = \mathbf{Q} \mathbf{x}$ . Moreover, a similarity transform of any operator  $\mathbf{T}$  from  $\mathbf{e}_i$  coordinates to  $\mathbf{d}_i$  coordinates is given by  $\mathbf{Q} \mathbf{T} \mathbf{Q}^\top$ .

We can also find the derivative of the directors as

$$\frac{\partial}{\partial s} \mathbf{d}_j = \frac{\partial}{\partial s} (\mathbf{Q}^\top \mathbf{e}_j) = \frac{\partial}{\partial s} (\mathbf{Q}^\top) \mathbf{e}_j = \frac{\partial}{\partial s} (\mathbf{Q}^\top) \mathbf{Q} \mathbf{d}_j =: \boldsymbol{\kappa} \times \mathbf{d}_j, \quad (\text{A4})$$

where we used the fact that  $\mathbf{Q}^\top \mathbf{Q} = \mathbb{I}$  implies that  $\frac{\partial}{\partial s} (\mathbf{Q}^\top) \mathbf{Q}$  is skew-symmetric. Furthermore, we have

$$\begin{aligned}
 \boldsymbol{\kappa} \times (\cdot) &= \dot{\mathbf{Q}}^\top \mathbf{Q}(\cdot) \\
 \mathbf{Q}(\boldsymbol{\kappa} \times (\cdot)) &= \mathbf{Q} \dot{\mathbf{Q}}^\top \mathbf{Q}(\cdot) \\
 (\mathbf{Q} \boldsymbol{\kappa}) \times (\mathbf{Q}(\cdot)) &= \mathbf{Q} \dot{\mathbf{Q}}^\top \mathbf{Q}(\cdot) \\
 \boldsymbol{\kappa}_b \times (\mathbf{Q}(\cdot)) &= \mathbf{Q} \dot{\mathbf{Q}}^\top \mathbf{Q}(\cdot) \\
 \boldsymbol{\kappa}_b^\times &= \mathbf{Q} \dot{\mathbf{Q}}^\top.
 \end{aligned} \tag{A5}$$
